# Supplementary material for: Convergence towards an Erd{\H o}s-R\'enyi graph structure in network contraction processes
Source: arXiv:2009.02890 ancillary file (2020-09-07)
Supplement: Supplementary file 1 [file Supp_Mat_Tishby2019.pdf]

# Supplemental Material:

## Convergence towards an asymptotic structure in network contraction processes

Ido Tishby, Ofer Biham and Eytan Katzav  
*Racah Institute of Physics, The Hebrew University, Jerusalem 91904, Israel*

### I. DETAILED DERIVATION OF THE MASTER EQUATION

Below we derive the master equation describing the temporal evolution of the degree distribution  $P_t(k)$ , during the contraction process of a network under different node deletion scenarios: random node deletion, preferential node deletion and propagating node deletion. In all these scenarios the number of nodes in the network at time  $t$  is  $N_t = N - t$ . The number of nodes of degree  $k$  at time  $t$  is denoted by  $N_t(k)$ , where

$$N_t = \sum_k N_t(k). \quad (\text{S1})$$

The degree distribution of the network at time  $t$  is given by

$$P_t(k) = \frac{N_t(k)}{N_t}. \quad (\text{S2})$$

#### A. Random node deletion

We first consider a network contraction scenario in which at each time step a random node is deleted from the network together with its links. To derive an equation for the time dependence of  $N_t(k)$  one needs to account for the primary effect of the deletion of a node of degree  $k$  and for the secondary effect in which nodes of degrees  $k$  and  $k+1$  lose a link due to the deletion of an adjacent node. The probability that the deleted node is of degree  $k$  is given by  $P_t(k)$ . Regarding the secondary effect, in case that the node deleted at time  $t$  is of degree  $k'$ , it affects  $k'$  other nodes, which lose one link each. Among these  $k'$  nodes, the probability of each one of them to be of degree  $k$  is given by  $kN_t(k)/[N_t\langle K \rangle_t]$ . Summing up over all the possible values of the degree  $k'$  of the deleted node and evaluating the expectation value of the number of nodes of degree  $k$  that are connected to the deleted node we obtain that the secondary effect on nodes of degree  $k$  is given by

$$\frac{d}{dt}N_t(k) = - \sum_{k'} \frac{N_t(k')}{N_t} \frac{k'kN_t(k)}{N_t\langle K \rangle_t} = - \frac{kN_t(k)}{N_t}. \quad (\text{S3})$$

The complete equation for the time dependence of  $N_t(k)$  is thus given by

$$\frac{d}{dt}N_t(k) = \frac{(k+1)}{N_t} [N_t(k+1) - N_t(k)]. \quad (\text{S4})$$

Using the relation  $P_t(k) = N_t(k)/N_t$  and the fact that  $dN(t)/dt = -1$ , we obtain the master equation

$$\frac{d}{dt}P_t(k) = \frac{1}{N_t} [(k+1)P_t(k+1) - kP_t(k)]. \quad (\text{S5})$$

#### B. Preferential node deletion

In the scenario of preferential node deletion, at each time step a node is selected for deletion with probability proportional to its degree. The equation describing the time dependence of  $N_t(k)$  should account for the probability that the deleted node is of degree  $k$  as well as for the secondary effect on other nodes of degrees  $k$  and  $k+1$ . The

probability that the node selected for deletion at time  $t$  will be of degree  $k$  is given by  $kN_t(k)/[N_t\langle K\rangle_t]$ . In case that the node selected for deletion at time  $t$  is of degree  $k'$  there are  $k'$  other nodes that will be affected, losing one link each. Among these  $k'$  nodes, the fraction of nodes of degree  $k$  is given by  $kN_t(k)/[N_t\langle K\rangle_t]$ . Summing up over all the possible values of the degree  $k'$  and evaluating the expected value for the number of nodes of degree  $k$  that are connected to the deleted node we obtain that the secondary effect on nodes of degree  $k$  is

$$\frac{d}{dt}N_t(k) = -\sum_{k'} \left[ \frac{k'N_t(k')}{N_t\langle K\rangle_t} \right] \left[ \frac{k'kN_t(k)}{N_t\langle K\rangle_t} \right] = -\frac{\langle K^2\rangle_t}{\langle K\rangle_t^2 N_t} kN_t(k). \quad (\text{S6})$$

This term appears with a negative sign when accounting for the loss of a link from a node of degree  $k$ , and with a positive sign when accounting for the loss of a link from a node of degree  $k+1$ . The complete equation for  $N_t$  ( $K=k$ ) is thus given by

$$\frac{d}{dt}N_t(k) = \frac{\langle K^2\rangle_t}{\langle K\rangle_t^2 N_t} [(k+1)N_t(k+1) - kN_t(k)] - \frac{k}{\langle K\rangle_t N_t} N_t(k). \quad (\text{S7})$$

Using the relation  $P_t(k) = N_t(k)/N_t$  and the fact that  $dN_t/dt = -1$ , we obtain the master equation

$$\frac{d}{dt}P_t(k) = \frac{\langle K^2\rangle_t}{\langle K\rangle_t^2 N_t} [(k+1)P_t(k+1) - kP_t(k)] - \frac{k - \langle K\rangle_t}{\langle K\rangle_t N_t} P_t(k). \quad (\text{S8})$$

### C. Propagating node deletion

The propagating node deletion scenario describes network contraction processes such as cascading failures and epidemics, in which the damage propagates from a deleted node to its neighbors. In this scenario, at each time step we delete a random neighbor of the node deleted in the previous step. In case that the last deleted node does not have any yet-undeleted neighbor, we pick a random node, select a random neighbor of this node for deletion and continue the process from there. The probability that the node deleted at time  $t$  will be of degree  $k'$  is given by  $kN_t(k')/[N_t\langle K\rangle_t]$ . One of these  $k'$  edges connects it to the node deleted in the previous time step and another edge connects it to the node to be deleted in the next time step. Apart from these two neighbors, there are  $k'-2$  neighbors that lose one link each upon deletion of a node of degree  $k'$ . Among the  $k'-2$  nodes, the expected fraction of nodes of degree  $k$  is given by  $kN_t(k)/[N_t\langle K\rangle_t]$ . Summing up over all the possible degrees  $k'$  of the node deleted at time  $t$ , we evaluate the expectation value for the number of nodes of degree  $k$  that are connected to the deleted node. The secondary effect on nodes of degree  $k$  is thus given by

$$\frac{d}{dt}N_t(k) = -\frac{\langle K^2\rangle_t - 2\langle K\rangle_t}{\langle K\rangle_t^2 N_t} kN_t(k). \quad (\text{S9})$$

This term appears with a negative sign when accounting for loss of a link from a node of degree  $k$ , and with a positive sign when accounting for a loss of a link from a node of degree  $k+1$ . The complete equation describing the time dependence of  $N_t(k)$  is thus given by

$$\frac{d}{dt}N_t(k) = \frac{\langle K^2\rangle_t - 2\langle K\rangle_t}{\langle K\rangle_t^2 N_t} [(k+1)N_t(k+1) - kN_t(k)] - \frac{k}{N_t\langle K\rangle_t} N_t(k). \quad (\text{S10})$$

Using the relation  $P_t(k) = N_t(k)/N_t$  and the fact that  $dN_t/dt = -1$ , we obtain the master equation

$$\frac{d}{dt}P_t(k) = \frac{\langle K^2\rangle_t - 2\langle K\rangle_t}{\langle K\rangle_t^2 N_t} [(k+1)P_t(k+1) - kP_t(k)] - \frac{k - \langle K\rangle_t}{\langle K\rangle_t N_t} P_t(k). \quad (\text{S11})$$

## II. THE TIME DERIVATIVE OF THE RELATIVE ENTROPY

In each one of the network contraction scenarios considered above, the degree distribution  $P_t(k)$  evolves in time according to the corresponding master equation. As a result, the relative entropy  $S_t$ , defined by

$$S_t = \sum_k P_t(k) \ln \left[ \frac{P_t(k)}{\pi_t(k)} \right], \quad (\text{S12})$$

also evolves as the network loses nodes and edges. The time derivative of  $S_t$  is given by

$$\frac{d}{dt} S_t = \sum_k \ln \left[ \frac{P_t(k)}{\pi_t(k)} \right] \frac{d}{dt} P_t(k) + \sum_k \left[ \frac{d}{dt} P_t(k) - \frac{P_t(k)}{\pi_t(k)} \frac{d}{dt} \pi_t(k) \right].$$

In each of the network contraction scenarios discussed above, the Poisson distribution  $\pi_t(k)$  is a fixed point, given by

$$\pi_t(k) = \frac{c_t^k}{k!} e^{-c_t}. \quad (\text{S13})$$

The time derivative of  $\pi_t(k)$  is given by

$$\frac{d}{dt} \pi_t(k) = -\frac{dc_t}{dt} \left( 1 - \frac{k}{c_t} \right) \pi_t(k). \quad (\text{S14})$$

Inserting these expressions in Eq. (S13), we find that the second term on the right hand side vanishes. As a result, the time derivative of the entropy is given by

$$\frac{d}{dt} S_t = \sum_k \ln \left[ \frac{P_t(k)}{\pi_t(k)} \right] \frac{d}{dt} P_t(k). \quad (\text{S15})$$

This is a general equation that applies to any network contraction scenario in which the Poisson distribution  $\pi_t(k)$  is a solution. In order to obtain a more specific equation for a given network contraction scenario, one should insert the expression for the derivative  $dP_t(k)/dt$  from the corresponding master equation into Eq. (S15).

## III. SUPPLEMENTAL FIGURE

In order to show that the convergence of contracting networks towards the ER structure is not limited to scale-free networks, we present in Fig. S1 results for the contraction of a random attachment network. In the random attachment model at each time step a new node is added to the network and connects randomly (rather than preferentially) to  $m$  of the existing nodes. For a seed network we use a complete graph of  $m + 1$  nodes. Unlike the BA network that exhibits a power-law degree distribution, the random attachment network has an exponential degree distribution. In the random attachment network  $\Gamma_0$  is positive, namely the network is assortative, unlike the BA network which is disassortative. It is found that both the relative entropy  $S_t$  and the degree-degree correlation function quickly decay, confirming the convergence towards the ER structure.

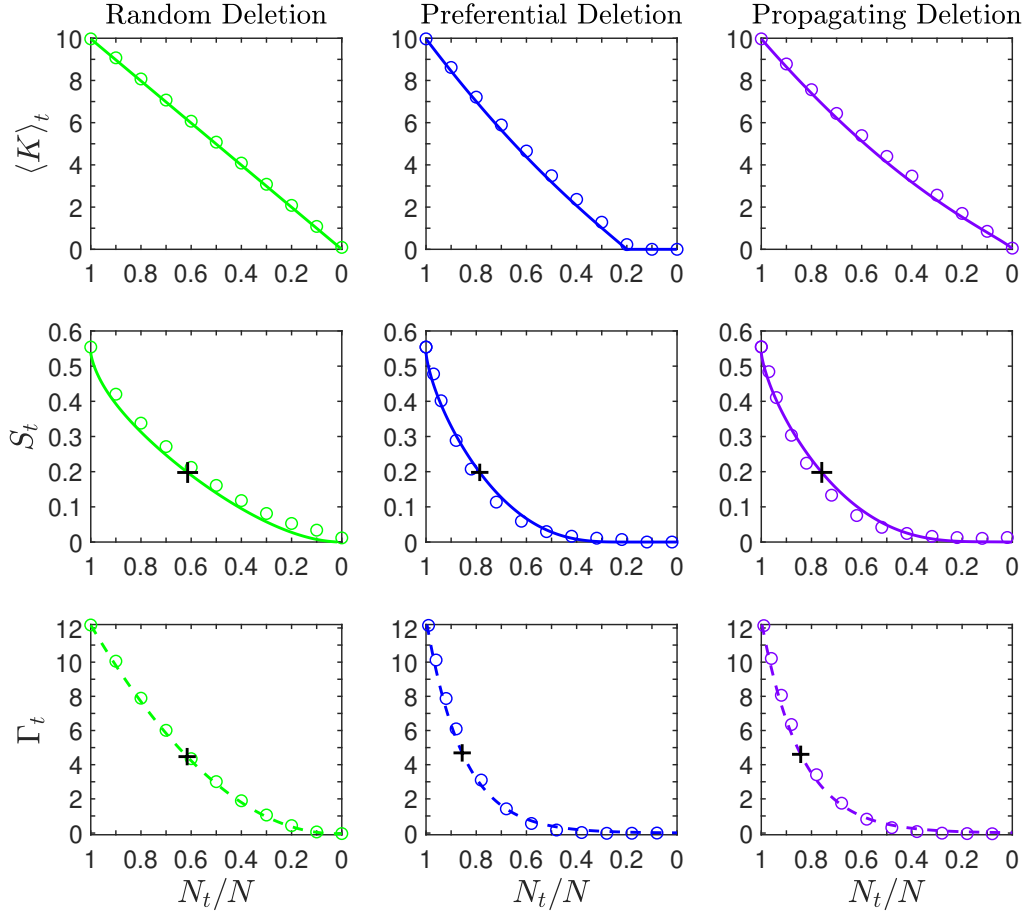

FIG. S1: The time dependence of the mean degree,  $\langle K \rangle_t$  (first row), the relative entropy  $S_t$  (second row) and the correlation function  $\Gamma_t$  (third row) for random deletion (left column), preferential deletion (middle column) and propagating deletion (right column) starting from a *random attachment* network with  $m = 5$  and size  $N = 1000$ . The results for  $\langle K \rangle_t$  and for  $S_t$ , obtained from numerical integration of the master equation (solid lines) are in very good agreement with computer simulations (circles). The simulation results for  $\Gamma_t$  (circles) are very well fitted by  $\Gamma_t \sim (N_t/N)^2$  for random deletion and by an exponential fit for preferential and for propagating deletion (dashed lines). The + symbols mark the points at which  $S_t$  and  $\Gamma_t$  decay to  $1/e$  of their initial values. In the case of random deletion this occurs around  $N_t/N \simeq 0.6$ . In the other two scenarios  $S_t$  is reduced to  $1/e$  of its initial value slightly below  $N_t/N \simeq 0.8$ , while  $\Gamma_t$  is reduced to  $1/e$  of its initial value slightly above  $N_t/N \simeq 0.8$ .
